# Supplementary material for: A Multi-day Needs-based Modeling Approach for Activity and Travel Demand Analysis
Source: arXiv:2312.15373 source file (2023-12-24)
Supplement: Supplementary file 2 [file AppendixIV.tex]

\section{E-Commerce Demonstration}\label{appendixIV:ecommerce_demonstration}

The input and parameters have been updated to demonstrate the ability of the model to capture e-commerce activity patterns. First, only one location, namely online, has been considered as the candidate location. No measure of size or attractiveness has been proposed for online shopping to the best of the authors' knowledge, and, instead of employment density, the attractiveness has been fixed to 100. Online shopping requires no travel, and therefore travel time and cost has been set to 0. The free time of both weekday and weekend days followed the same distribution described in Section \ref{section:monte_carlo_exp}. Size measures have not been used for this exercise, and retail employment and zonal area have not been generated. In terms of the individual parameters, $\gamma$ has been fixed to 1.4, assuming a larger depletion rate over the weekend. The scale parameter $\mu$ of the joint location and participation choice has been decreased to 0.1, assuming a less determinant decision. The rest of the parameters have the same value or distribution as in Table \ref{table:mc_test_param}. Figure \ref{fig:ecommerce_demonstration} shows the daily participation and distribution of activity durations by day of week, among the 1500 individuals. Thus, Monday has the highest e-commerce activity participation, which resembles the reported pattern of e-commerce activity \citep{statista_2017}. 
\begin{figure}[htpb]
    \centering
    \includegraphics[width=6.3 in]{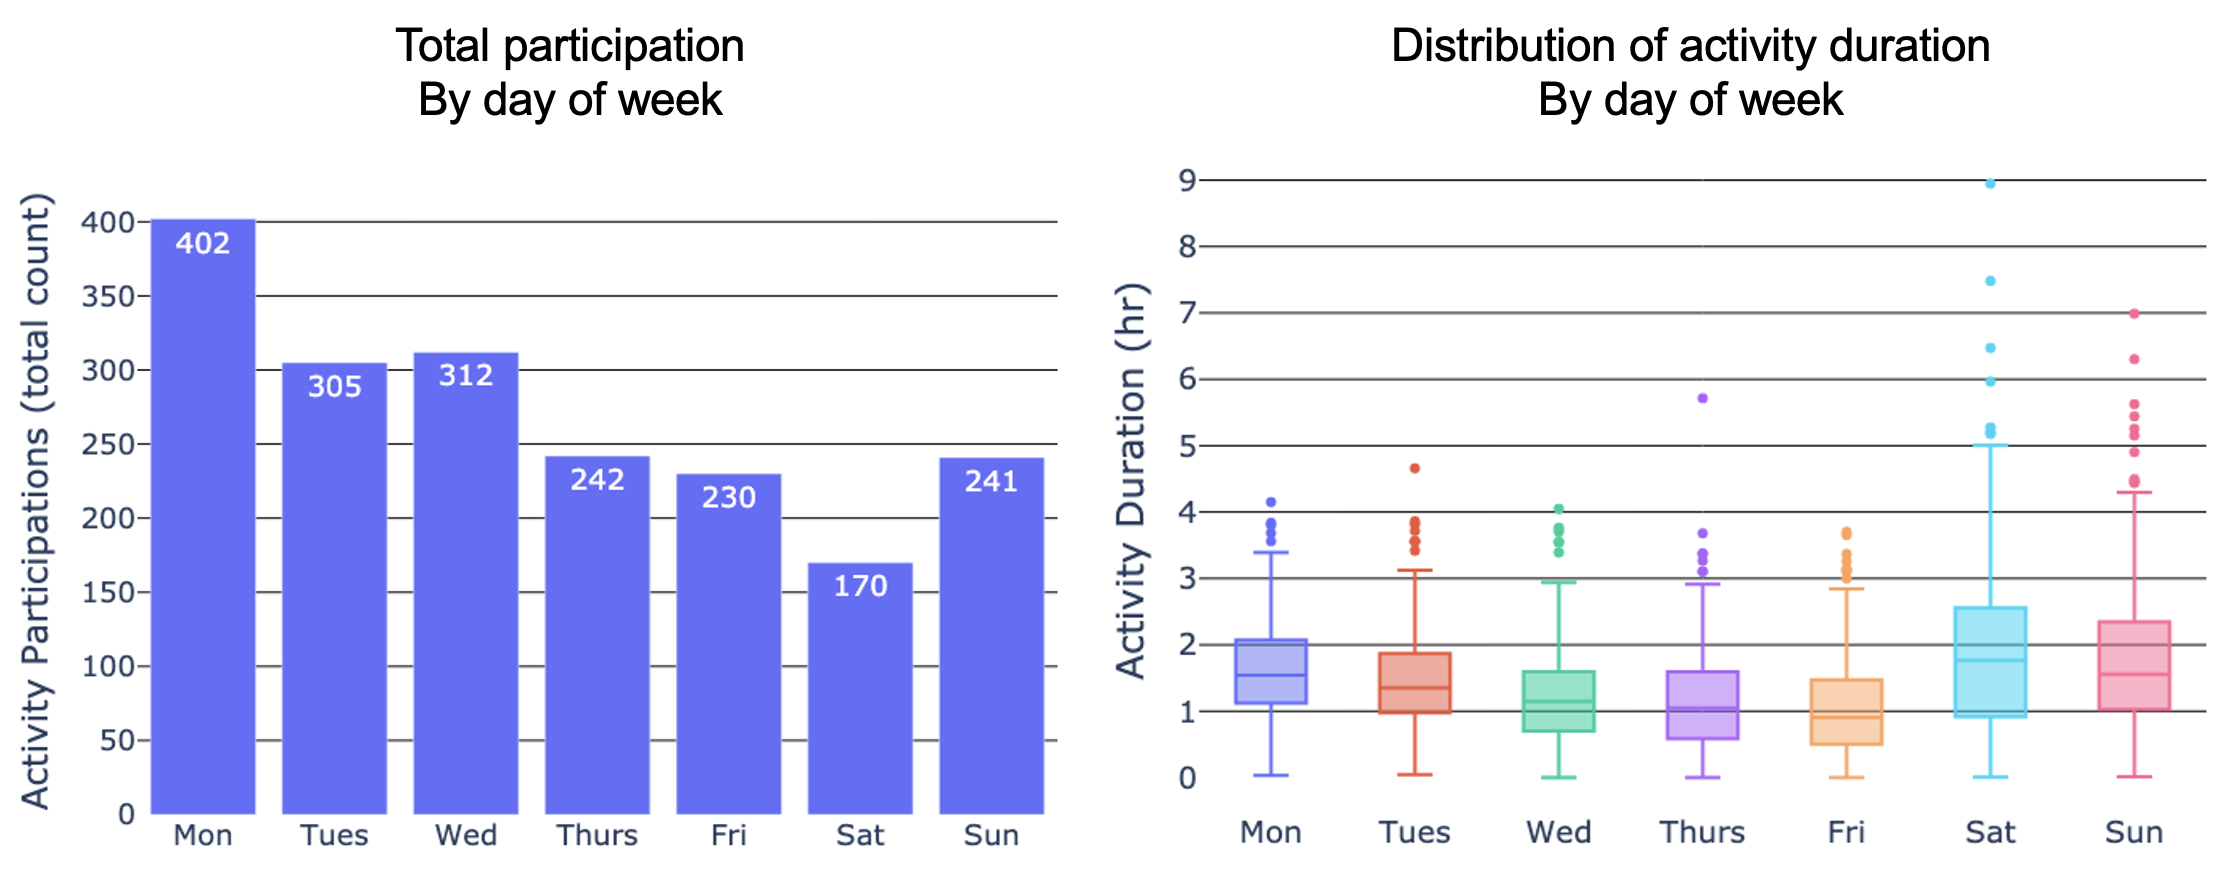}
    \caption{Pattern of Synthesized Sample for E-Commerce Demonstration}
    \label{fig:ecommerce_demonstration}
\end{figure}
